# Supplementary material for: Machine Learning of Temperature-dependent Chemical Kinetics Using Parallel Droplet Microreactors
Source: arXiv:2512.19416 source file (2026-09-21)
Supplement: Supplementary file 1 [file supplementary_material.pdf]

# Supporting Information:
# Machine Learning of Temperature-dependent Chemical Kinetics Using Parallel Droplet Microreactors

Mamoru Saita, Yutaka Hori*

Department of Applied Physics and Physico-Informatics,
Faculty of Science and Technology, Keio University, Japan
{mamosaita64, yhori}@keio.jp

## Supplementary Note 1: Immobilization of droplets

The image of the entire chamber at the beginning of the experiment ($t = 0$ min), corresponding to Fig. 2B, is shown in Fig. S1. The colored lines in the figure represent the trajectories of the droplet centers tracked over 180 min. Droplets without the trajectories correspond to those that could not be continuously tracked during the time course and were therefore excluded from the analysis. Figure S1 illustrates that the displacement of most detected droplets remains within approximately one droplet radius (100 µm) throughout the observation window (180 min), indicating stable immobilization of the droplets.

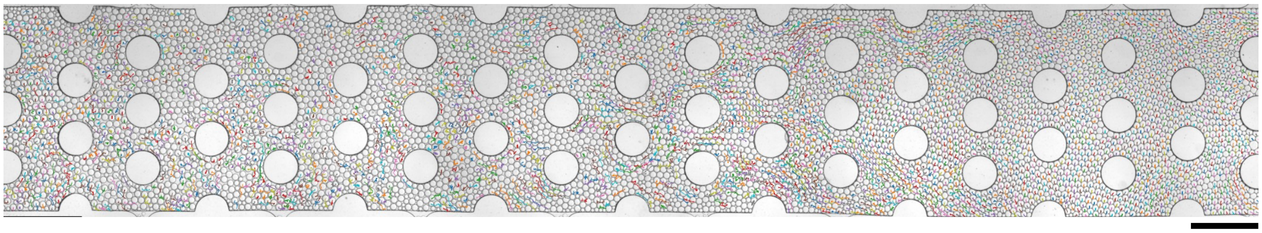

Figure S1: Trajectory analysis of droplets immobilized under a temperature gradient. Bright-field image of the entire chamber at 0 min is overlaid with the trajectories of droplets tracked for 180 min. Scale bar represents 1 mm.

# Supplementary Note 2: Calibration of DNA thermometer

The calibration curve of the DNA thermometer in Fig. 2C was obtained by fitting the averaged fluorescence intensities of droplets measured at each temperature to a sigmoidal function using nonlinear least-squares optimization. Curve fitting was performed with the `curve_fit` function of the SciPy library [1] in Python, which employs the Levenberg–Marquardt (LM) algorithm for unconstrained minimization.

The fluorescence intensity $F$ of the DNA thermometer as a function of temperature $T$ was modeled as

$$F(T) = \frac{a}{1 + b\,\exp\bigl(c\,(T + d)\bigr)} + e, \tag{1}$$

where $a$, $b$, $c$, $d$, and $e$ are fitting parameters. The fitted parameters are summarized in Table S1.

Table S1: Fitted parameters of the DNA thermometer calibration curve obtained by nonlinear least-squares fitting

| **Parameter** | **Symbol** | **Fitted value** |
|---|---|---|
| Amplitude | $a$ | 7659 |
| Scaling factor | $b$ | 3.045 |
| Slope coefficient | $c$ | $-0.1950$ |
| Temperature shift | $d$ | $-35.39$ |
| Offset | $e$ | 544.0 |

# Supplementary Note 3: Neural ODE model for stationary temperature gradient

Figure S2 shows Neural ODE prediction against all observed data under stationary temperature gradient, corresponding to Fig. 3E, where only a subset of the time points is displayed. A strong linear correlation indicates that the Neural ODE model successfully reproduces the enzyme kinetics under various static temperature conditions.

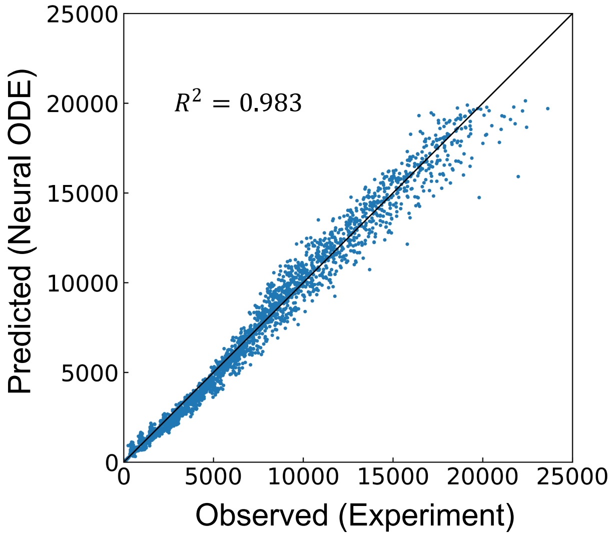


Figure S2: Neural ODE prediction plotted against all test data under stationary temperature gradient.

## Supplementary Note 4: Ordinary Differential Equation (ODE) model

To benchmark the data-driven Neural ODE model against a conventional physics based model, we constructed an ODE model of the enzymatic reaction based on physics laws. The model parameters were then optimized to fit the experimental data taken under the stationary temperature gradient (Fig. 3).

The substrate and product concentrations were modeled based on the Michaelis–Menten kinetics by

$$\frac{dS(t)}{dt} = -\frac{1}{B}\frac{V_{\max}(T)\,S(t)}{K_m + S(t)}, \tag{2}$$

$$\frac{dP(t)}{dt} = \frac{V_{\max}(T)\,S(t)}{K_m + S(t)}, \tag{3}$$

where $P(t)$ represents the measured fluorescence intensity corresponding to the product concentration, $S(t)$ denotes a latent variable corresponding to the substrate, $T$ is the absolute temperature, and $B$ and $K_m$ are constants. To reflect the temperature-dependent catalytic activity of the enzyme, the term $V_{\max}(T)$, which is the maximum rate of product formation, was defined as a function of the absolute temperature $T$.

The dependence of $V_{\max}(T)$ on temperature was modeled according to the Arrhenius-type relationship by

$$\ln V_{\max}(T) = \alpha\frac{1}{T} + \beta, \tag{4}$$

where $\alpha$ and $\beta$ are constants reflecting the activation energy and the constant factor, respectively.

The product fluorescence exhibited a gradual increase during the first 10 minutes until the droplet temperature was stabilized (see Fig. 3A). A steady nearly linear increase was then observed between 10 and 30 minutes, implying that the reaction rate was saturated. Thus, assuming that the the substrate concentration was much higher than the Michaelis-Menten constant $K_m$ between 10 and 30 minutes, $V_{\max}(T)$ was determined from the slope of the droplet fluorescence intensity.

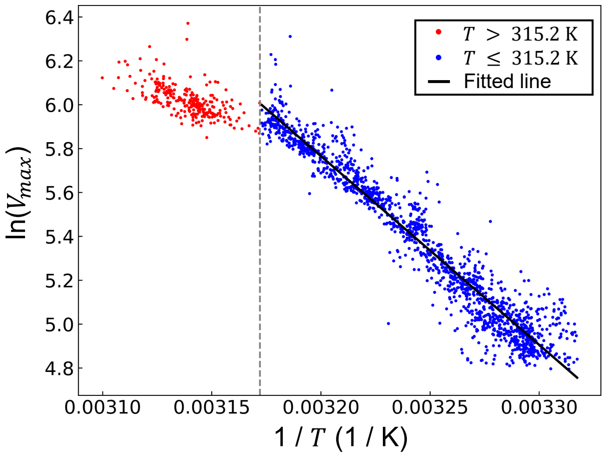


Figure S3: Linear fitting of $\ln(V_{\max})$ with $1/T$ at $t = 30$ min below the transition temperature $T_{\text{break}} = 42.1\,°\text{C}$.

Fig. S3 shows the experimentally measured $\ln(V_{\max})$, where $\ln(V_{\max})$ decreases almost linearly with $1/T$ in the low-temperature region around 40 ° C (313 K; $1/T > 0.00319$), which is consistent with eq. (4), whereas the slope was not maintained at higher temperatures. This deviation could be due to the faster substrate depletion within the first 10 minutes at high temperatures, where the enzymatic reaction proceeds rapidly and no longer maintains a constant reaction rate. To examine the temperature range over which the linear relationship remains valid, linear fitting was performed for progressively extended temperature windows,

starting from 35 $^\circ$ C (308 K; $1/T = 0.003246$) and increasing the upper bound in 0.1 $^\circ$ C increments. For each temperature window, the mean squared error (MSE) between the observed and fitted $\ln(V_{\max})$ values was computed. The minimum of MSE was achieved for the temperature range below $T_{\text{break}} = 42.1\,^\circ\text{C}$ (315.2 K; $1/T = 0.003173$). Within this windows, linear regression yielded coefficients $\alpha = -8600.09$ and $\beta = 33.29$ (Fig. S3).

The remaining parameters, $K_m$ and $B$, were determined by fitting the ODE to all time-series data with $T > T_{\text{break}}$. Specifically, the parameters $K_m$ and $B$ were searched over a grid of candidate values ranging from $5 \leq K_m \leq 25$ (step size 5) and $100 \leq B \leq 900$ (step size 200). The minimizer of the mean squared error (MSE) between the simulated and observed trajectories was determined as $K_m = 10$ and $B = 500$ (Fig. S4A).

Finally, the ODE model was evaluated on the test dataset to assess its predictive performance (Fig. 3F). The fitted time-series data corresponding to Fig. 3F is shown in Fig. S4B. Figure S4C shows ODE prediction against all observed data under dynamic temperature gradient, corresponding to Fig. 3F, where only a subset of the time points is displayed. The ODE predictions tend to underestimate the experimental output, indicating that the simple ODE formulation does not fully capture temperature-dependent enzyme dynamics across the entire range.

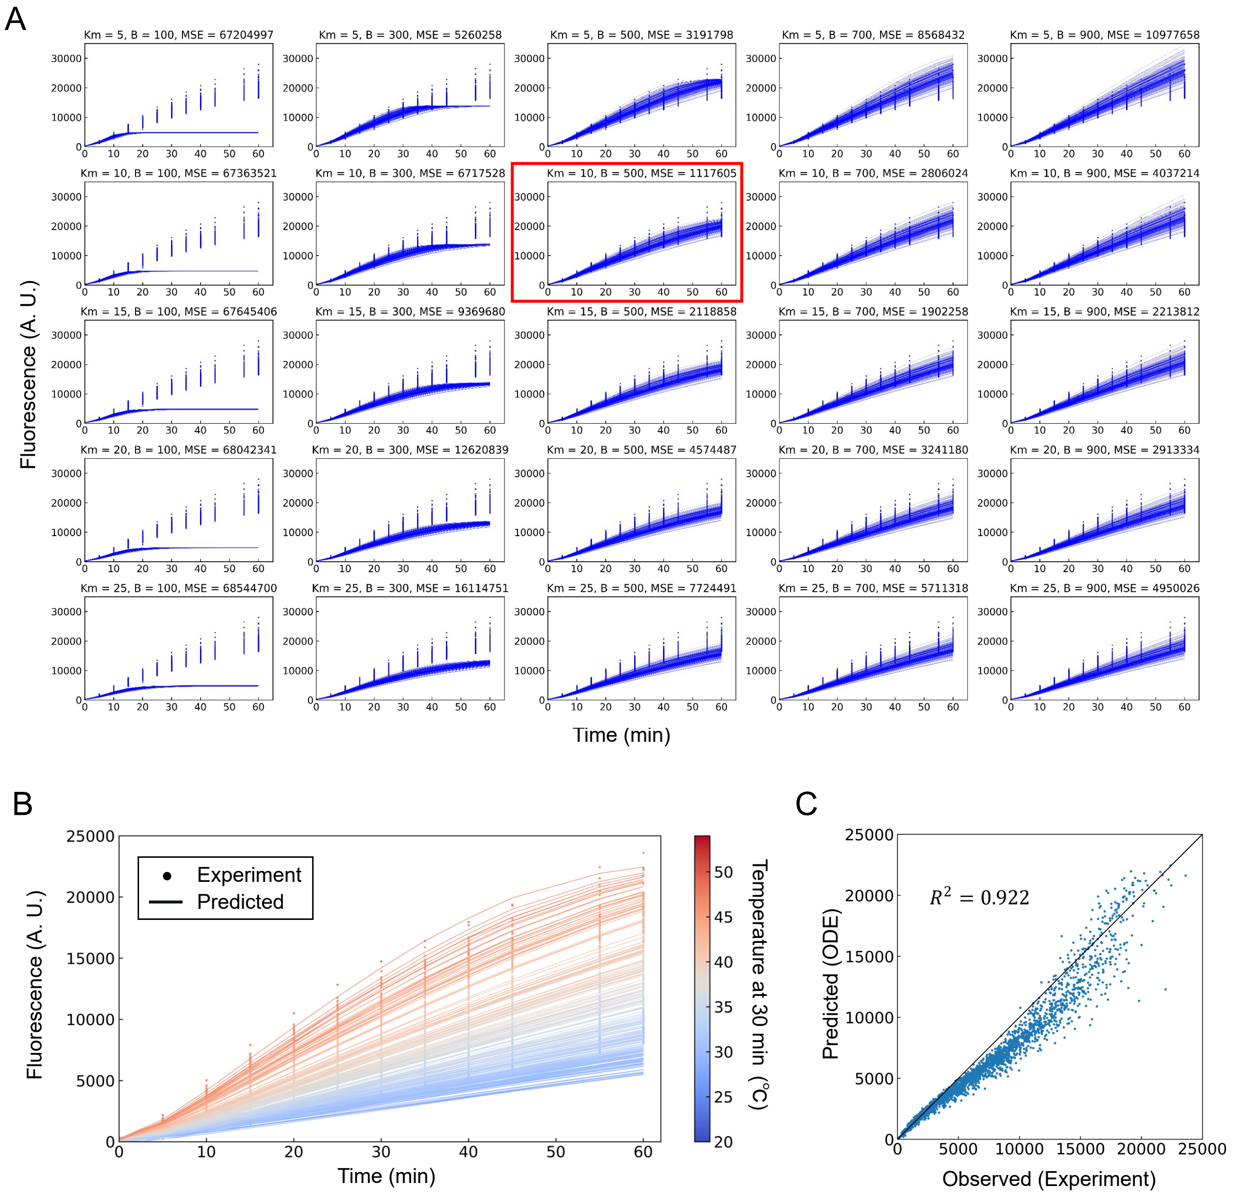


Figure S4: (A) Results of the grid search over candidate values of the parameters $K_m$ and $B$ using training dataset. The parameter combination $K_m = 10$ and $B = 500$, highlighted by the red box, yields the smallest mean squared error (MSE). (B) Time-series of product fluorescence compared with prediction by ODE model with test dataset. (C) Predicted fluorescence obtained by ODE plotted against experimental data with test dataset.

## Supplementary Note 5: Neural ODE model for dynamic temperature gradient

Figure S5 shows Neural ODE prediction against all observed data under dynamic temperature gradient, corresponding to Fig. 4F, where only a subset of the time points is displayed. A strong linear correlation indicates that the Neural ODE model successfully reproduces the enzyme kinetics under various dynamic temperature conditions.

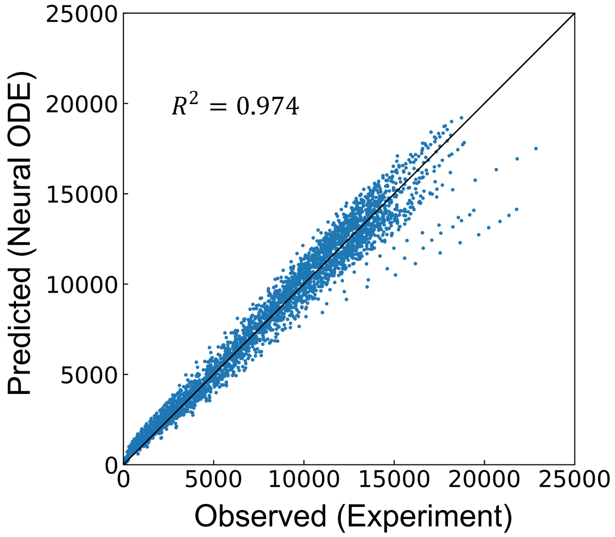


Figure S5: Neural ODE model prediction plotted against all test data under dynamic temperature gradient.

## Supplementary Note 6: Sequence of DNA Thermometer

The following DNA sequence was used as the DNA thermometer. The strand was labeled with a fluorescent dye (TAMRA) at the 5′ end and a quencher (BHQ2) at the 3′ end. The DNA sequence used in this study was adopted from that reported in literature [2].

Table S2: Sequence of DNA thermometer

| Name | Sequence |
|---|---|
| DNA thermometer | TAMRA-GGGTTTTTTTTTTTTTTTT-<br>-TTTTTTTTTTTTTTTTTAACCC-BHQ2 |

## Supplementary Note 7: Temperature control system

The temperature control system used in this study was constructed using two Peltier elements (TEC1-12708, Thermonamic Electronics) and a single-board computer Raspberry Pi (Raspberry Pi® 4 Model B, Raspberry Pi Ltd.) as the main controller. For the purpose of feedback control, temperature was measured with two platinum resistance thermometers (SDT101BXN100DF, KOA), each placed near one end of the glass slide. A schematic overview of the entire temperature control circuit is shown in Fig. S6A. Each platinum resistance thermometer was embedded in a PDMS block as shown in Fig. S6B, and the PDMS block was attached to the surface of the Peltier element (Fig. S6C). A four-terminal sensing method was used to measure the voltage across each platinum resistance thermometer, and the analog voltage signal was digitized using an analog-to-digital converter (ADS122U04IPW, Texas Instruments) before being input to the Raspberry Pi. The temperature was estimated from the measured resistance according to the resistance–temperature characteristics specified in the datasheet of the platinum resistance thermometer.

The temperature of each Peltier element was controlled by applying voltage to the Peltier elements through an H-bridge circuit driven by a motor driver (TB67H450FNG, Toshiba), which enabled both heating and cooling by switching the current direction according to control commands from the Raspberry Pi.

Temperature regulation was achieved by pulse-width modulation (PWM) control implemented on the Raspberry Pi, in which the duty ratio was dynamically adjusted according to the deviation between the target and measured temperatures. The PWM frequency was set to 100 Hz, and the proportional–integral (PI) control was employed to ensure stable convergence to the desired temperature.

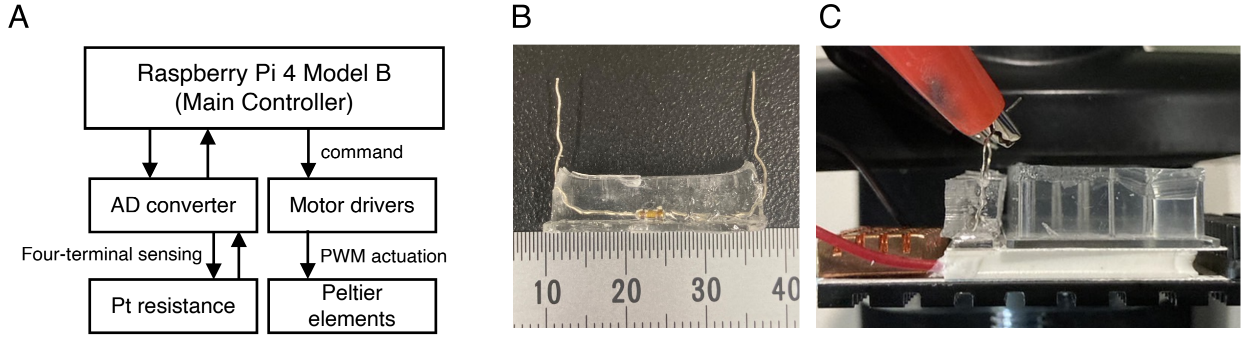


Figure S6: (A) A schematic overview of the entire temperature control circuit. (B) A platinum resistance thermometer encapsulated in a PDMS block. (C) Side view of a platinum resistance thermometer placed on the surface of the Peltier element.

## References

[1] Pauli Virtanen, Ralf Gommers, Travis E. Oliphant, Matt Haberland, Tyler Reddy, David Cournapeau, Evgeni Burovski, Pearu Peterson, Warren Weckesser, Jonathan Bright, Stéfan J. van der Walt, Matthew Brett, Joshua Wilson, K. Jarrod Millman, Nikolay Mayorov, Andrew R. J. Nelson, Eric Jones, Robert Kern, Eric Larson, C J Carey, İlhan Polat, Yu Feng, Eric W. Moore, Jake VanderPlas, Denis Laxalde, Josef Perktold, Robert Cimrman, Ian Henriksen, E. A. Quintero, Charles R. Harris, Anne M. Archibald, Antônio H. Ribeiro, Fabian Pedregosa, Paul van Mulbregt, and SciPy 1.0 Contributors. SciPy 1.0: Fundamental Algorithms for Scientific Computing in Python. *Nature Methods*, 17:261–272, 2020.

[2] Noel L. Goddard, Grégoire Bonnet, Oleg Krichevsky, and Albert Libchaber. Sequence dependent rigidity of single stranded DNA. *Physical Review Letter*, 85:2400–2403, 2000.
